# Supplementary material for: SCL with Theory Constraints
Source: arXiv:2003.04627 source file (2020-10-22)
Supplement: Supplementary file 1 [file paper-appendix.tex]

\section{Saturation}

\begin{definition}
  Let $N$ and $U$ be sets of clauses. 
  Then $N \cup U$ is a \emph{saturated} clause set if SCL(T) cannot learn new clauses from $N \cup U$, i.e., there exists no sequence of rule applications following a state $(\epsilon;N;U;B;0;\top)$ that contains the rule Conflict.
\end{definition}

\begin{theorem} \label{theo:saturationdetection}
  Let $N$ and $U$ be sets of clauses and $B$ be a sequence 
  of constants such that $|B| \geq 2 \cdot \max_{C\in N \cup U} |\vars(C)|$. 
  Then $N \cup U$ is a saturated clause set iff 
  there exists a regular $\SCLT$ run starting in state $(\epsilon;N;U;B;0;\top)$ that does not use rule Grow, explores all possible trail prefixes for $B$, and does not encounter a single conflict.
\end{theorem}
\begin{proof}
$\Rightarrow$: 
Assume $N \cup U$ is saturated, then by definition all regular $\SCLT$ runs starting in $(\epsilon;N;U;B;0;\top)$ encounter no conflicts. 
This also includes all runs that do not use rule Grow and explore all possible trail prefixes for $B$.

$\Leftarrow$: 
Assume $N \cup U$ is not saturated.
Then there exists a regular $\SCLT$ run
$(\epsilon;N;U;B;0;\top)
    \Rightarrow_\SCLT^*
    \ldots
    \Rightarrow^{\text{Conflict}}_{\SCLT} (M;N;U;B';k;(\Lambda'\parallel D)\cdot\sigma)$.
Due to Corollary~\ref{corol:resolve-after-conflict}, $\forgd(M) = M',L\rho^{(\Lambda\parallel  C\lor L)\cdot\rho}$, 
$D\cdot\sigma' = (D' \lor L')\cdot\sigma$, $L\cdot\rho = \comp(L'\cdot\sigma)$, $(\Lambda'\parallel D) \in N \cup U$, and there exists 
$(\Lambda\parallel  C \lor C_1 \lor L) \in N \cup U$ such that $(\Lambda\parallel  C \lor C_1 \lor L) \cdot \rho = (\Lambda\parallel  C\lor L)\cdot\rho$. 
Next we create a run that can be executed purely over the constants in $B$ but still leads to a conflict. 
To this end, we assume w.l.o.g. that $\cdom(\rho) \cup \cdom(\sigma) \subseteq B$. 
This is possible because $|\cdom(\rho) \cup \cdom(\sigma)| \leq |\vars(\Lambda\parallel  C\lor C_1 \lor L)| + |\vars(\Lambda'\parallel  D)| \leq |B|$. 
Moreover, we assume that $L_1, \ldots, L_n$ are the complements of the ground literals occurring in $C\cdot\rho$ and $D'\cdot\sigma$. 
For our new run over $B$, we start from state $(\epsilon;N;U;B;0;\top)$ and add the literals $L_1^1, \ldots, L_n^n$ via decisions on the trail. 
Note that we cannot encounter a conflict by just deciding the literals $L_1, \ldots, L_n$ 
because (i)~a regular run must apply conflict greedily, (ii)~the trail $M'$ also contained the literals $L_1, \ldots, L_n$, and (iii)~in the last run conflict was only applicable after $L\cdot\rho$ was propagated on top of $M'$. 
However, we will encounter one of two cases that will lead to a conflict over $B$: 
Case 1: The conditions of a regular run force us to stop our sequence of decisions at a prefix trail $M^* =L_1^1, \ldots, L_i^i$ with $i < n$ because there are two clauses $C^*, D^* \in N \cup U$ such that we can propagate $L^* \cdot \rho^*$ from $C^* \cdot \rho^*$ and receive a conflict in $D^* \cdot\sigma^*$. 
Hence, we have a regular run over $B$ without rule Grow that leads to a conflict.
Case 2: We are able to decide all literals $L_1, \ldots, L_n$. 
From the trail $M^* =L_1^1, \ldots, L_n^n$ we can propagate $L\cdot\rho$ via the clause $(\Lambda\parallel C\lor C_1 \lor L) \in N \cup U$ and the substitution $\rho$. 
This turns $(\Lambda'\parallel  D) \cdot \sigma$ into a conflict. 
Hence, we have a regular run over $B$ without rule Grow that leads to a conflict.
In both cases, all regular $\SCLT$ runs starting in state $(\epsilon;N;U;B;0;\top)$ that do not use rule Grow and explore all possible trail prefixes for $B$ must encounter this trail prefix and therefore also this conflict.
\end{proof}

\section{Old}

A \emph{many-sorted signature} $\sig = (\sorts,\opers, \Pi)$ is a triple consisting of a finite non-empty 
set $\sorts$ of \emph{sort symbols}, a non-empty set
$\opers$ of \emph{operator symbols} (also called \emph{function symbols}) over $\sorts$ and a set 
$\Pi$ of \emph{predicate symbols}. Every operator symbol $f \in \opers$ has a unique sort declaration 
$f:S_1 \times \ldots \times S_n \rightarrow S$, indicating the sorts of arguments (also called \emph{domain sorts}) 
and the \emph{range sort} of $f$, respectively, for some $\tenum{S}{n}, S \in \sorts$ 
where $n \geq 0$ is called the \emph{arity} of $f$, also denoted with $\arity(f)$. An operator 
symbol $f \in \opers$ with arity 0 is called a \emph{constant}. Every predicate symbol $P \in \Pi$ has a unique sort declaration
$P \subseteq S_1 \times \ldots \times S_n$. A predicate symbol $P \in \Pi$ with arity 0 is called
a \emph{propositional variable}. As usual, sorts are assumed to be inhabited. For every sort $S \in \sorts$ there must be at least one 
constant $a \in \opers$ with range sort $S$.

Given a signature $\sig = (\sorts,\opers, \Pi)$ and a variable set $\varset$, containinng infinitly many
variables for each sort in $\sorts$, terms are defined in the usual way. $\term_{S}(\sig,\varset)$ denotes
all terms of sort $S$ and $\term_{S}(\sig)$ the set of all ground terms of sort $S$. Note that $\term_{S}(\sig)$
is non-empty for any $S$ because sorts are inhabited.

Literals and clauses are defined in the usual way where $f, g, h$ denote function symbols,
$a, b, c$ constants, $w, x, y, z$ variables, $t, s$ terms, $P, Q, R$ predicates, $A, B$ atoms,
$L, K, H$ denote literals, $C, D$ denote clauses, and $N$ denotes a clause set. For substitutions
we write $\sigma, \delta, \rho$.
The complement of a literal is denoted by the function $\comp$. As usual, clauses are disjunctions
of literals with implicitely universally quantified variables.

Let $\sig = (\sorts, \opers, \Pi)$ be a signature with set of sorts $\sorts$, operator set $\opers$ and predicate set $\Pi$. 
A \emph{$\sig$-algebra} $\sigval$, also called \emph{$\sig$-interpretation}, is a mapping that assigns
(i)~a non-empty carrier set $S^{\sigval}$ to every sort $S \in \sorts$, 
so that $(S_1)^{\sigval} \cap (S_2)^{\sigval} = \emptyset$ for any distinct sorts $S_1, S_2 \in \sorts$,
(ii)~a total function $f^{\sigval} : (S_1)^{\sigval} \times \ldots \times (S_n)^{\sigval} \rightarrow (S)^{\sigval}$ to 
every operator $f \in \opers$, $\arity(f)=n$ where $f: S_1 \times \ldots \times S_n \rightarrow S$,
(iii)~a relation $P^{\sigval} \subseteq ((S_1)^{\sigval} \times \ldots \times (S_m)^{\sigval})$ to every predicate symbol $P \in \Pi$, $\arity(P)=m$.
The semantic entailment relation $\models$ is defined in the usual way.

Given a first-order \emph{theory} $\theory$ consists of a many-sorted signature  $\sig$ and
a non-empty set of $\sig$-algebras $\modset$, i.e., $\theory = (\sig,\modset)$. 

Let $\theory^B = (\sig^B,\modset^B)$ be a many-sorted theory, called the \emph{background theory}
and $\sig^B$ the \emph{background signature}.
Let $\sig^F$ be a many sorted signature with $\opers^B\cap\opers^F=\emptyset$, $\sorts^B\subset\sorts^F$, 
called the \emph{foreground signature} or \emph{free signature}.
Let $\sig^H = (\sorts^B\cup\sorts^F, \opers^B\cup\opers^F)$ be the union signature
and $N$ be a set of clauses over $\sig^H$, and $\theory^H = (\sig^H, N)$ called a \emph{hierarchic theory}.
A pair $\hspec = (\theory^H, \theory^B)$ is called a \emph{hierarchic specification}.

For the rest we assume a hierarchic specification $\hspec = (\theory^H, \theory^B)$.
We abbreviate  $\models_{\theory^B} \phi$ ($\models_{\theory^H} \phi$) with $\models_B \phi$ ($\models_H \phi$),
meaning that $\phi$ is valid in the respective theory.
Terms, atoms, literals build over $\sig^B$ are called \emph{pure background terms}, 
\emph{pure background atoms}, and
\emph{pure background literals}, respectively. 
Non-variable terms, atoms, literals build over $\sig^F$ are called \emph{free terms}, \emph{free atoms}, 
\emph{free literals}.  A variable of sort $S\in (\sorts^F\setminus\sorts^B)$ is also called 
a  \emph{free variable} and a  \emph{free term}.
Any term of some sort $S\in \sorts^B$ built out of $\sig^H$ is called a \emph{background term}.
A substitution $\sigma$ is called \emph{simple} if $x_S\sigma\in\term_S(\sig^B,\varset)$ for
all $S\in\sorts^B$.

Given a hierarchic specification $\hspec = (\theory^H, \theory^B)$,
$\theory^B = (\sig^B,\modset^B)$, $\theory^H = (\sig^H, N)$,
a $\sig^H$-algebra $\inta$ is called \emph{hierarchic} if $\inta|_{\sig^B}\in\modset^B$.
A hierarchic algebra $\inta$ is called a \emph{model of a hierarchic specification} $\hspec$, 
if $\inta\models N$.

A term $t$ is called \emph{abstracted} with respect to a hierarchic specification $\hspec = (\theory^H, \theory^B)$,
if $t\in\term_S(\sig^B,\varset)$ or $t\in\term_T(\sig^F,\varset)$ for some $S\in\sorts^B$, $T\in\sorts^B\cup\sorts^F$.
A clause is called \emph{abstracted} of all its literals are abstracted.

Abtraction can be obtained from any hierarchic specification by exhaustive application of the below abstraction rule.

\begin{definition}
  HERE WE ALREADY ASSUME THAT $\opers^F$ only contains infinitely many function symbols of sorts $S\in\sorts^B$.
\end{definition}

\bigskip
\shortrules{Abstraction}{$N\disjun\{C\lor [\neg]P(\ldots,t_i,\ldots)\}$}{$N\cup\{C\lor x_s \not\approx t_i \lor [\neg]P(\ldots,x_S,\ldots)\}$}{provided 
  $t_i$ is a non-variable term of sort $S$, and $t_i\in\term_S(\sig^B,\varset)$}{ABSTR}{12}

We consider a compact background theory $\mathcal T^B = (\Sigma^B,\mathcal C^B)$ with equality where $\Sigma^B = (\mathcal S^B, \Omega^B)$ is called background
signature and $\mathcal C^B$ is a set of term generated algebras over $\Sigma^B$. A \emph{hierarchic specification}\cite{kruglov2012superposition} is a
pair $\mathcal H = (\mathcal T^F, \mathcal T^B)$ such that $\mathcal T^F = (\Sigma^F, N)$ where $N$ is a finite clause set over $\Sigma^F$ and $\Sigma^F = (\mathcal S^F, \Omega^F)$
is a signature with $\Omega^B \cap \Omega^F = \emptyset$ and $\mathcal S^B \subsetneq \mathcal S^F$. $\mathcal T^F$ is called foreground theory, terms,
atoms and literals are called \emph{pure background} if they only contain operators in $\Omega^B$.
In this work we assume that function symbols in $\Sigma^F\setminus \Sigma^B$ are constants of sorts in $\mathcal S^F \setminus \mathcal S^B$
so all terms and literals of a background sort are pure.

For simplicity we only consider one background sort $S \in \mathcal S^B$ and assume that all predicates in
$\Sigma^F$ all range over $S$. Other finite sorts in $\Sigma^F$ can be easily simulated in this setting;
equality beyond the scope of this paper.

Substitutions $\sigma, \tau$ are total mappings from variables to terms, where
 $\dom(\sigma) := \{x \mid x\sigma\neq x\}$ is finite and $\cdom(\sigma)
 := \{ t\mid x\sigma = t,x\in\dom(\sigma)\}$.
Given a hierarchic specification a substitution $\sigma$ is called \emph{simple} if it maps variable of background sort to pure background terms, that is if $ x_S\sigma \in T_S(\Sigma^B,\mathcal X_S)$, in this paper we only consider simple substitutions.
Their application is extended to literals, clauses,
and sets of such objects in the usual way.

\begin{definition}[Hierarchic Entailment]
  Given a hierarchic specification $\mathcal H = (\mathcal T^F,\mathcal T^B)$,
  $\mathcal T^B = (\Sigma^B,\mathcal C^B)$,  $\mathcal T^F = (\Sigma^F, N)$
  we define a hierarchic algebra for $\mathcal H$ as an algebra $\mathcal A$
  for the theory $\mathcal T^F$ such that the restriction
  $\mathcal A\restriction_{\Sigma^B}\in\mathcal C^B$. $\mathcal A$ is a model
  of $\mathcal H$ if it is a hierarchic algebra and $\mathcal A\models N$.
  Hierarchic entailment $\models_{\mathcal H}$ is defined as usual entailment
  restricted to hierarchic algebras.
\end{definition}

\begin{definition}[Subsumed Constrained Clauses]
  Given two ground constrained clauses $\Lambda_1\|C_1$
  and $\Lambda_2\|C_2$ we say that $\Lambda_1\|C_1$
  \emph{subsumes} $\Lambda_2\|C_2$
  if $\Lambda_1 \subseteq \Lambda_2$ and $C_1 \subseteq C_2$.

  Given two constrained clauses $\Lambda_1\|C_1$
  and $\Lambda_2\|C_2$ we say that $\Lambda_1\|C_1$ \emph{subsumes}
  $\Lambda_2\|C_2$ with respect to a set $B$ of arithmetic constants
  if for all ground clauses $\Lambda'_2\|C'_2 \in \mGnd_B(\Lambda_2\|C_2)$
  there is a clause $\Lambda'_1\|C'_1 \in \mGnd_B(\Lambda_1\|C_1)$
  such that $\Lambda'_1 \subseteq \Lambda'_2$ and $C'_1\subseteq C'_2$.

  Given a state $(M;N;N;B;k;s)$ we say that
  a constrained clause $\Lambda\|C$ is
  subsumed in $(M;N;U;B;k;s)$ if $\Lambda\|C$
  is subsumed in $N \cup U$ with respect to B.
\end{definition}

Let $L_1,\ldots,L_n$ be a finite enumeration of all foreground ground literals from
with respect to a finite set of constants $B$, without
duplicates. We call this a $\sig^{\hspec}_B$ \emph{enumeration}.

% \bigskip
% \shortrules{Decide-Restart}
% {$(M,L\sigma^{\Lambda\|C\lor L\cdot\sigma},M';N;U;B;k;\top)$}
% {$(M,K\delta^{i+1};N;U;B;i+1;\top)$}
% { provided $M$ is of level $i$, $K\delta$ is undefined in $M$,
%   $|K|$ occurs in $N\cup U$, $\cdom(\delta)\subseteq B$,
%   and $K\delta$ does not create a conflict
% }{\SCLT}{11}

\bigskip
\shortrules{Decide-Restart}
{$(M,L,M';N;U;B;k;\top)$}
{$(M,(K\delta)_n^{i+1};N;U;B;i+1;\top)$}
{ provided $M$ is of level $i$, $L$ is not a restart literal,
  $K\delta$ is the literal of maximal index of the  $\sig^{\hspec}$ enumeration
  with respect to $B$, such that $|K|$ occurs in $N\cup U$,
  $\cdom(\delta)\subseteq B$, $K\delta$ does not create a conflict and
  $K\delta$ is undefined in $M$.
}{\SCLT}{11}

\bigskip
\shortrules{Decide-Retry}
{$(M,L_n^{i+1},M';N;U;B;k;\top)$}
{$(M,(K\delta)_{m}^{i+1};N;U;B;i+1;\top)$}
{ provided $M$ is of level $i$, $K\delta$ is undefined in $M$,
  $|K|$ occurs in $N\cup U$, $\cdom(\delta)\subseteq B$,
  $K\delta$ does not create a conflict,
  and $m>0, m<n$.
}{\SCLT}{11}

\begin{lemma}[$\SCLT$ Simulates Hierarchic Factoring] \label{lemm:simres-factor}
  Let $N$ be a clause set, $\Lambda\|C\lor H\lor H'$
  a non-tautological clause with unifiable literals $H$ and $H'$.
  There is a run starting from the state
  $(\epsilon;N;\emptyset;0;B;\top)$ where the first
  learned clause is $(\Lambda\|C'\lor H)\eta$
  where $\eta=\mMGU(H,K)$ if $B$
  contains at least $|\vars(\Lambda\|C)| + |\vars(H)|$ foreground constants.
\end{lemma}
\begin{proof}
  Let $\{L_1,\dots,L_k\} = C\eta$ and let $\rho$
  be a grounding of $C\lor H\lor H'$ injective on the literals of $(C\lor H\lor H')\eta$ where $|\vars(\Lambda\|C)| + |\vars(H)|$ constants suffice.
  By applying Decide $k$ times we can reach a state
  \[
    (K_1^1\rho,\ldots,K_k^k\rho;
    N;\emptyset;B;k;\top)
  \]
  with $K_i = \comp(L_i)$, from which we can apply rule Conflict
  to $C\eta\rho$ resulting in
  \[
    (K_1^1\rho,\ldots,K_k^k\rho;
    N;\emptyset;B;k;
    \Lambda\|C\cdot\eta\cdot\rho).
  \]
  Now we can factorize $H$ and $H'$, deriving
  \[
    (K_1^1\rho,\ldots,,K_k^k\rho;N;
    \emptyset;B;k;
    (\Lambda\|C'\lor H)\eta\cdot\rho)
  \]
  and, finally, backtrack and learn $(\Lambda\|C'\lor H)\eta$.
\end{proof}

%%%%%%%%%%%%%%%%%%%%%%%%%%%%%%%%%%%%%%%%%%%%%%%%%%%%%%%%%%%%%%%%%%%%%%%%%%%%%%%
\begin{lemma}\label{thm:well-founded}
  Let $(C_i)_{i\in\mathbb{N}}$ an infinite
  sequence of distinct ground clauses where
  duplicated literals are not implicitly eliminated.
  Assume that the set $\mathcal L = \bigcup_{i\in\mathbb{N}}C_i$
  only has finitely many distinct literals.
  Then there is an index $j$ such that $C_j$
  is subsumed in $\{C_k|0\le k < j\}$.
\end{lemma}
\begin{proof}
  Assume by contradiction that all $C_j$ are not subsumed in
  $M'_j=\{C_k|0\le k < j\}$. Let $n = |\mathcal L|$ with
  $\mathcal L = \{L_1,\dots,L_n\}$, we encode each clause
  $C_i$ as a tuple $q_i=(m^i_1,\dots,m^i_n)\in\mathbb{N}^n$
  where $m^i_k$ is the multiplicity of $L_k$ in $C_i$,
  on $\mathbb N^n$ we take a partial order $\le$
  defined the point-wise partial order of $\mathbb{N}^n$.
  We have that $q^i\le q^j$ if and only if $C_i$ subsumes $C_j$.

  Now consider the set $M_i = \{q_j|0 \le j \le i\}$,
  $q_i$ is minimal in $M_i$ if and only if $C_i$
  is not subsumed in $M'_i$.
  Now we define $M = \bigcup_{i\in\mathbb{N}} M_i$,
  by Dickson's lemma\cite{dickson1913finiteness}
  the set of minimal points of $M$ is finite.
  This means that for all but finitely many indexes $i$
  there exists a $j$ such that $q_j < q_i$ and since we have
  assumed that no $C_i$ is subsumed in $M'_i$ we must also
  have $i < j$. This implies the existence of a strictly
  decreasing subsequence $(q_{k_i})_{i\in\mathbb{N}}$
  which is in contradiction with the
  well-foundedness of $(\mathbb{N}^n,\le)$.
\end{proof}

%%%%%%%%%%%%%%%%%%%%%%%%%%%%%%%%%%%%%%%%%%%%%%%%%%%%%%%%%%%%%%%%%%%%%%%%%%%%%%%
%%%%%%%%%%%%%%%%%%%%%%%%%%%%%%%%%%%%%%%%%%%%%%%%%%%%%%%%%%%%%%%%%%%%%%%%%%%%%%%
\begin{lemma}
  Starting from a well-formed state $(M;N;U;B;k;\top)$
  conflict search terminates if Grow is applied finitely often.
\end{lemma}
\begin{proof}
  The rules that can be applied in conflict search are: Propagate,
  Decide, Grow, Decide-Restart, Decide-Retry, and Conflict.
  Conflict always terminates conflict search as no conflict search rule
  can be applied immediately following a Conflict.
  In the following we assume that Conflict is never invoked.
  Assume that after the last application of Grow we have $B'$ as
  set of available constants and that $l$ is the number of distinct
  foreground literals appearing in $\mGnd_{B'}(N)$.
  Given a trail $M$, we consider the sequence of foreground literals in $M$
  \[\forgd(M) = L_1,\dots,L_n\]
  we define $\mu(M)= [m_1,\dots,m_n,(1,3),\ldots,(1,3)]\in (\mathbb N\times\mathbb N)^l$
  where $|\mu(M)|=l$ and $m_i=(1,2)$ if $L_i=K^{\Lambda\|C\cdot\sigma}$
  is a propagated literal, $m_i=(1,1)$ if $L_i=K^k$ is a decision literal,
  and  $m_i=(0,n)$ if $L_i=K_n^k$ is a restart literal.
  We consider the lexicographical order $<_{\text{lex}}$ on $(\mathbb N\times\mathbb N)^l$ induced by the lexicographical order on $\mathbb N\times\mathbb N$  and show that
  every application of Propagate, Decide, Decide-Restart, and Decide-Retry all decrease
  the measure $\mu$.
  Given a $M$ with $\mu(M)= [m_1,\dots,m_n,3,\ldots,3]$ both Propagate
  and Decide produce a state $M'$ whose measure is in the form
  $\mu(M)= [m_1,\dots,m_n,(1,3),\ldots,(1,3)]$ with $m=(1,2)$ if we applied
  Propagate and $m=(1,1)$ if Decide was applied instead
  while the first $n$ components remained unchanged.
  In both cases $m<(1,3)$ and so $\mu(M') <_{\text{lex}} \mu(M)$.
  Given a $M$ with $\mu(M)= [m_1,\dots,m_n,3,\ldots,3]$ an application of
  Decide-Restart or Decide-Retry produces a trail $M'$ with measure
  $\mu(M')=[m_1,\dots,m_{k-1},(0,n),3,\dots,3]$ with $1\le k\le n$,
  where the $k$-th component of $\mu(M)$ was either $(1,2)$, $(1,1)$, or  $(0,n')$ with $n'>n$. In all cases we have $\mu(M') <_{\text{lex}} \mu(M)$.
  % where the $k$-th literal in $\forgd(M)$ is not a restart literal
  % and the $k$-th literal in $\forgd(M')$ is a restart literal and
  %all preceding literals remained unchanged.
  By since $<_{\text{lex}}$ on $(\mathbb N\times\mathbb N)^l$ is a well-order
  every conflict search must terminate.
\end{proof}

%%%%%%%%%%%%%%%%%%%%%%%%%%%%%%%%%%%%%%%%%%%%%%%%%%%%%%%%%%%%%%%%%%%%%%%%%%%%%%%
\begin{definition}[Reasonable Run]
  A sequence of $\SCLT$ rules applications is called a \emph{reasonable run}
  if it is a fair run, the rule Conflict has precedence on all
  other rules, both Resolve and then Skip have precedence over Backtrack,
  and Decide never causes a conflict.
%  and, if rule Decide-Restart and Decide-Retry are always used on the right-most
%  valid literal.
\end{definition}
%%%%%%%%%%%%%%%%%%%%%%%%%%%%%%%%%%%%%%%%%%%%%%%%%%%%%%%%%%%%%%%%%%%%%%%%%%%%%%%

\begin{example}[Reasonable run]\Todo{}
  % With a trail $M,L\sigma^{\Lambda\|C\cdot\sigma},M',(L')^k_m,M''$
  % If $m>0$ we cannot apply Decide-Restart on $L\sigma^{\Lambda\|C\cdot\sigma}$
  % because to its right there is a literal on which we can apply Decide-Retry,
  % $(L')^k_m$.
  % Similarly on a trail $M,(L')^k_m,M',L\sigma^{\Lambda\|C\cdot\sigma},M''$
  % Assuming $m>0$ we cannot apply Decide-Retry on $(L')^k_m$
  % because to its right there is a literal on which we can apply Decide-Restart,
  % $L\sigma^{\Lambda\|C\cdot\sigma}$.
\end{example}
%%%%%%%%%%%%%%%%%%%%%%%%%%%%%%%%%%%%%%%%%%%%%%%%%%%%%%%%%%%%%%%%%%%%%%%%%%%%%%%

\begin{lemma}\label{lemm:retry-non-red}
  Let $N$ be a set of constrained clauses.
  Then clauses learned in a $\SCLT$ reasonable run from starting state $(\epsilon;N;\emptyset;B;0;\top)$ are not
  redundant.
\end{lemma}
\begin{proof}
  Consider the following fragment of a derivation learning a clause:
  \begin{align*}
    &\Rightarrow^{\text{Conflict}}_{\SCLT} &(M;N;U;B;k;\Lambda_0\|C_0\cdot\sigma_0)\\
    &\Rightarrow^{\{\text{Skip, Fact., Res.}\}^*}_{\SCLT} &(M';N;U;B;k;\Lambda_n\|C_n\cdot\sigma_n)\\
    &\Rightarrow^{\text{Backtrack}}_{{\SCLT}}&(\epsilon;N;U\cup\{\Lambda_n\|C_n\};B;0;\top).
  \end{align*}
  Let $\prec$ be the $\hspec$ order induced by $M$. We prove that $\Lambda_n\sigma_n\|C_n\sigma_n$
  is not redundant with respect to $\prec$ , $B$, and $(N\cup U)$.
  By soundness of hierarchic resolution $(N\cup U) \models \Lambda_n\|C_n$
  and $\Lambda_n\sigma_n\|C_n\sigma_n$ is false under both $M$ and $M'$.
  For a proof by contradiction, assume there is a
  $N'\subseteq\mGnd_B(N\cup U)^{\preceq \Lambda_n\sigma_n\|C_n\sigma_n}$
  such that $N'\models_\hspec\Lambda_n\sigma_n\|C_n\sigma_n$.
  As $\Lambda_n\sigma_n\|C_n\sigma_n$ is false under $M$,
  there is a ground constrained clause $\Lambda'\|C'\in N'$
  with $\Lambda'\|C' \preceq \Lambda_n\sigma_n\|C_n\sigma_n$,
  and all literals from $C'$ are defined in $M$ and false by the definition of $\prec$.
  Furthermore, $\backgd(M)\land\Lambda'$ is satisfiable.
  Now since decision literals cannot initiate conflicts we must have $M=M_0,L\sigma^{\Lambda\|C\cdot\sigma}$
  and both $C_0\sigma_0$ and $C'$ contain the literal $\comp(L\sigma)$, but by exhaustive application of Resolve
  before backtrack we know that $C_n\sigma_n$ has no occurrences of  $\comp(L\sigma)$.
  Now we have $\Lambda_n\sigma\|C_n\sigma \prec L\sigma \preceq \Lambda'\|C'$;
  in contradiction with the existence of $N'\subseteq\mGnd_B(N\cup U)^{\preceq \Lambda_n\sigma_n\|C_n\sigma_n}$
  such that $N'\models_\hspec\Lambda_n\sigma_n\|C_n\sigma_nx$.
\end{proof}

\begin{proof}
  Consider the following fragment of a derivation learning a clause:
  \begin{align*}
    &\Rightarrow^{\text{Conflict}}_{\SCLT} &(M;N;U;B;k;\Lambda_0\|C_0\cdot\sigma_0)\\
    &\Rightarrow^{\{\text{Skip, Fact., Res.}\}^*}_{\SCLT} &(M';N;U;B;k;\Lambda_n\|C_n\cdot\sigma)\\
    &\Rightarrow^{\text{Backtrack}}_{{\SCLT}}&(\epsilon;N;U\cup\{\Lambda_n\|C_n\};B;0;\top).
  \end{align*}
  Let $\prec$ be the $\hspec$ order induced by $M$. We prove that $\Lambda_n\sigma\|C_n\sigma$
  is not redundant with respect to $\prec$ , $B$, and $(N\cup U)$.
  By soundness of hierarchic resolution $(N\cup U) \models \Lambda_n\|C_n$
  and $\Lambda_n\sigma\|C_n\sigma$ is false under both $M$ and $M'$.
  For a proof by contradiction, assume there is a
  $N'\subseteq\mGnd_B(N\cup U)^{\preceq \Lambda\sigma\|C\sigma}$
  such that $N'\models_\hspec\Lambda\sigma\|C\sigma$.
  As $\Lambda_n\sigma\|C_n\sigma$ is false under $M$,
  there is a ground constrained clause $\Lambda'\|C'\in N'$ with $\Lambda'\|C' \preceq \Lambda_n\sigma\|C_n\sigma$,
  and all literals from $C'$ are defined in $M$ and false by the definition of $\prec$.
  Furthermore, $\backgd(M)\land\Lambda'$ is satisfiable.

  Consider the following fragment of a derivation learning a clause:
  \[
    \begin{aligned}
      &\Rightarrow^{\text{Conflict}}_{\SCLT}\\      &(M;N;U;B;k;\Lambda_0\|C_0\cdot\sigma_0)\\
      &\Rightarrow^{\{\text{Skip, Fact., Res.}\}^*}_{\SCLT}\\
      &(M';N;U;B;k;\Lambda\|C\cdot\sigma)\\
      &\Rightarrow^{\text{Backtrack}}_{{\SCLT}}
    \end{aligned}
  \]
  By soundness of resolution $N\cup U \models \Lambda\|C$
  and $\Lambda\sigma\|C\sigma$ is false under both $M$ and $M'$.
  We prove that $\Lambda\sigma\|C\sigma$ is non-redundant in $N\cup U$.

  Since all literals and clauses needed for this proof
  are obtained from literals and clauses appearing in
  $(M;N;U;B;k;\Lambda_0\|C_0\cdot\sigma_0)$ and
  by combining them with normal operations and unification
  we never run the risk of exhausting the set $B$ of constants
  during conflict resolution. Indeed computing the $\mMGU$ between literals
  or constrained clauses never requires introducing new constants,
  in particular $\cdom(\mMGU(\sigma,\delta))\subseteq\cdom(\sigma)\cup\cdom(\delta)$.
  We also know from the preconditions on the rule Backtrack that $k>0$.

  Assume there is a
  $S\subseteq\mGnd_B(N\cup U)^{\preceq \Lambda\sigma\|C\sigma}$
  \st $S\models_\hspec\Lambda\sigma\|C\sigma$.
  As $\Lambda\sigma\|C\sigma$
  is false under $M$ we also have
  that there is a constrained clause $D\in S$
  that is also false under $M$.

  Let $M''$ be the difference between $M'$ and $M$,
  that is $M = M',M''$, we distinguish two cases
  depending on whether $M''$
  contains or not any first order literal.

  If $M''$ contain a first order literal then $\Lambda\sigma\|C\sigma$ does
  not contain the rightmost first order literal of $M$ and
  since $D\prec \Lambda\sigma\|C\sigma$ neither does $D$.
  So at a previous point in the derivation there must have been
  a state such that $D$ was false under the current trail but was not
  chosen as conflict instance, a contradiction to the exhaustive
  application of Conflict.

  If $M''$ contains no foreground literals
  then the rightmost foreground literal $L$ of $M$
  is in $M'$. Without loss of generality we assume
  that conflict resolution start with enough Skip
  applications to reach the trail $M_0=M_1,L$.
  We distinguish two sub-cases according to whether $L$
  % the rightmost literal in $M$
  is the result of Propagation or a Decision.

  $L$ cannot be the result of a Decide-Retry or of a Decide-Restart
  because these rules can only create trails that do not initiate conflicts,
  in contradiction with $L$ being the rightmost foreground literal.

  If the rightmost literal of $M_0=M_1,L^k$ is a decision literal,
  then $D$ must be false under $M_0$ and undefined under $M_1$,
  due to Conflict having an higher precedence than Decide.
  Moreover since Propagation has precedence over Decide
  we know $D$ has at least two undefined foreground
  literals of level $k$. By the precondition of Backtrack
  we know that $C\sigma$  has at most one literal of level $k$
  in contradiction with $D\prec C\sigma$.

  If $M_0=M_1,L^{\Lambda'\|C'\cdot\delta}$
  then, then from the precondition of Backtrack,
  exactly one literal in $C\sigma$ is of level
  $k$ and all other literals, if any, are of level at most $k-1$.

  %%%%%%%%%%%%%%%%%%%%%%%%%%%%%%%%%%%%%%%%%%%%%%%%%%%%%%%%%%%%%%%%%%%%%%%%%%%%%
  %%%%%%%%%%%%%%%%%%%%%%%%%%%%%%%       %       %%%%%%%%%%%%%%%%%%%%%%%%%%%%%%%
  %%%%%%%%%%%%%%%%%%%%%%%%%%   Retry Restart Case   %%%%%%%%%%%%%%%%%%%%%%%%%%
  %%%%%%%%%%%%%%%%%%%%%%%%%%%%%%%%%%         %%%%%%%%%%%%%%%%%%%%%%%%%%%%%%%%%%
  %%%%%%%%%%%%%%%%%%%%%%%%%%%%%%%%%%%%%   %%%%%%%%%%%%%%%%%%%%%%%%%%%%%%%%%%%%%
  %%%%%%%%%%%%%%%%%%%%%%%%%%%%%%%%%%%%%%%%%%%%%%%%%%%%%%%%%%%%%%%%%%%%%%%%%%%%%
  %%%%%%%%%%%%%%%%%%%%%%%%%%%%%%%%%%%%%%%%%%%%%%%%%%%%%%%%%%%%%%%%%%%%%%%%%%%%%

  Suppose $M=M_0,K^k,\Lambda'\sigma',L'\sigma'^{\Lambda'\|C'\cdot\sigma'}$,
  we separate by cases on what literal
  $H$ was in that position before $K$

  Assume $D$ is false in $M$ and that the only foreground
  literal of level $k$ in $D$ is $\comp(L'\sigma')$.

  Claim: every useful trail was already tested on the literal $H$\\
  Claim: if $D$  has only one literal of level $k$, then $D$ also
  caused a conflict under $H$ or a preceding literal

  Consider the literal $J$ that was in that position before the
  application of Restart-Decide.
  If
  if $DD$ does not contain

  if $K=\xi(m)$ was a

  If $L$ is a retry then. Not possible

\end{proof}
\Todo{Check that in the enumeration of literals for Decide-Retry both positive and negatives literals are adequately covered}
\Todo{Decide-Restart should also remove the Background constraints introduced by propagations}

%%%%%%%%%%%%%%%%%%%%%%%%%%%%%%%%%%%%%%%%%%%%%%%%%%%%%%%%%%%%%%%%%%%%%%%%%%%%%%%
\begin{example}
  $B = \{a\}$,
  \[
    N=\left\{
      \begin{aligned}
        &\lnot C(x),\\
        &C(x)\lor\lnot B(x),\\
        % &x>0\|C(x)\lor B(x)\lor\lnot E,\\
        % &E\lor A,\\
        &x < 0\|\lnot E\lor A(x)\lor A(x)\lor B(x),\\
        &x < 0\|\lnot E\lor A(x)\lor C(x),\\
      \end{aligned}
  \right\}
  \]

\[\lnot C(a),\lnot B(a), a > 0\]
\end{example}
%%%%%%%%%%%%%%%%%%%%%%%%%%%%%%%%%%%%%%%%%%%%%%%%%%%%%%%%%%%%%%%%%%%%%%%%%%%%%%%
%%%%%%%%%%%%%%%%%%%%%%%%%%%%%%%%%%%%%%%%%%%%%%%%%%%%%%%%%%%%%%%%%%%%%%%%%%%%%%%
%%%%%%%%%%%%%%%%%%%%%%%%%%%%%%%%%%%%%%%%%%%%%%%%%%%%%%%%%%%%%%%%%%%%%%%%%%%%%%%
%%%%%%%%%%%%%%%%%%%%%%%%%%%%%%%%%%%%%%%%%%%%%%%%%%%%%%%%%%%%%%%%%%%%%%%%%%%%%%%
%%%%%%%%%%%%%%%%%%%%%%%%%%%%%%%%%%%%%%%%%%%%%%%%%%%%%%%%%%%%%%%%%%%%%%%%%%%%%%%
%%%%%%%%%%%%%%%%%%%%%%%%%%%%%%%%%%%%%%%%%%%%%%%%%%%%%%%%%%%%%%%%%%%%%%%%%%%%%%%
%%%%%%%%%%%%%%%%%%%%%%%%%%%%%%%%%%%%%%%%%%%%%%%%%%%%%%%%%%%%%%%%%%%%%%%%%%%%%%%

\bigskip
\shortrules{Decide-Retry}
{$(M,K^{i+1},M';N;U;B;k;\top)$}
{$(M,K'\delta^{i+1};N;U;B;i+1;\top)$}
{ provided $M$ is of level $i$, $K'\delta$ is undefined in $M$,
  $|K'|$ occurs in $N\cup U$, $\cdom(\delta)\subseteq B$,
  $K'\delta$ does not create a conflict,
  and $K'\delta \prec K$ according to some
  \textit{a priori} defined total order $\prec$ on the literals of $\mGnd_B(N)$.
}{\SCLT}{11}

%%%%%%%%%%%%%%%%%%%%%%%%%%%%%%%%%%%%%%%%%%%%%%%%%%%%%%%%%%%%%%%%%%%%%%%%%%%%%%%

%%%%%%%%%%%%%%%%%%%%%%%%%%%%%%%%%%%%%%%%%%%%%%%%%%%%%%%%%%%%%%%%%%%%%%%%%%%%%%%
\begin{example}[Marco's Example]
  \[
  N = \left\{
  \begin{aligned}
  x + y = 0 \|& P(x,y)\\
  u>v \land u+v=1 \land x<y \land x+y=z \land x'<y' \land x'+y'=z+1 \|& \lnot P(x,y) \lor  P(u,v) \lor P(x',y')\\
  x<y \land x+y=2 \land u'>v' \land u'+v'=1 \|& \lnot P(x,y) \lor P(u',v')\\
  \end{aligned}
  \right\}
  \]
\end{example}

\begin{example}[Marco's Example on Models Construction (modified)]
\[
N = \left\{
\begin{aligned}
x = 0 \land y = 0 \|& \lnot P(x,y)\\
u \le x \land x \le y \land y \le w \|& \lnot P(x,y) \lor P(u,w)\\
u < x \land x > y \land y < w \|& P(x,y) \lor P(u,w)\\
\end{aligned}
\right\}
\]

$N$ entails $0 \le x \land x \le y \land y \le 1 \| \lnot P(x,y)$ and $0 < x \land x > y \land y < 1 \| P(x,y)$

A possible trail for \SCLT on $N$ is:
\[a = 0, b = 1, \lnot P(a,b), a \le c, c \le d, d \le b, \lnot P(c,d), c < e, e > f, f < d, P(e,f) \]
from which we can extract the candidate representation:
\[\begin{gathered}
  \exists abcdef. \forall xy. a = 0 \land b = 1 \land a \le \land c \le d \land d \le b \land c < e \land e > f \land f < d \land \\ \left( P(x,y) \leftrightarrow \left( \lnot \left( x = 0 \land y = 1 \right) \land \lnot \left( a \le x \land x \le y \land y \le b \right) \land \left( c < x \land x < y \land y < d \right) \right)
\right)\end{gathered}\]

\end{example}

\begin{example}[Marco's Example on Models Construction (modified v2)]
\[
N = \left\{
\begin{aligned}
x = 0 \land y = 0 \|& \lnot P(x,y)\\
u \le x \land x \le y \land y \le w \|& \lnot P(x,y) \lor P(u,w)\\
u < x \land x \le y \land y < w \|& P(x,y) \lor P(w,u)\\
\end{aligned}
\right\}
\]

$N$ entails $0 \le x \land x \le y \land y \le 1 \| \lnot P(x,y)$ and $u < 0 \land 0 \le 1 \land 1 < w \| P(w,u)$

A possible trail for \SCLT on $N$ is:
\[a = 0, b = 1, \lnot P(a,b), a \le c, c \le d, d \le b, \lnot P(c,d), e < c, c \le d , d < f, P(f,e) \]
from which we can extract the candidate representation:
\[\begin{gathered}
\exists abcdef. \forall xy. a = 0 \land b = 1 \land a \le \land c \le d \land d \le b \land c < e \land e > f \land f < d \land \\ \left( P(x,y) \leftrightarrow \left( \lnot \left( x = 0 \land y = 1 \right) \land \lnot \left( a \le x \land x \le y \land y \le b \right) \land \left( y < c \land d < x \right) \right)
\right)\end{gathered}\]

\end{example}

\begin{example}
\[
N = \left\{
\begin{aligned}
x = 0 \|& P(x)\\
u=1 \land x' = x+1 \|& \lnot P(x) \lor  Q(u) \lor P(x')\\
x=2 \land u=1 \|& \lnot P(x) \lor Q(u)\\
\end{aligned}
\right\}
\]
\end{example}

\begin{example}
\[
N = \left\{
\begin{aligned}
x = 0 \|& P(x)\\
u=1 \land x' = x+1 \|& \lnot P(x) \lor  Q(u) \lor P(x')\\
x=2 \|& \lnot P(x)\\
u'=1  \|& \lnot Q(u')\\
\end{aligned}
\right\}
\]
\end{example}

\begin{example}
\[
N = \left\{
\begin{aligned}
x = 0 \|& P(x)\\
u=1 \land x' = x+1 \|& \lnot P(x) \lor  Q(u) \lor P(x')\\
u'=1  \land x=2 \|& \lnot P(x)\lor\lnot Q(u')\\
\end{aligned}
\right\}
\]
\end{example}

\begin{definition}[(Strong) Consistency]
  Let  $K = [\neg] P(b_1,\ldots,b_n)$ be a ground literal.
  We say that $K$ is \emph{consistent} with a trail $M$, if $M,K$ is satisfiable.
  We say that $K$ is \emph{strongly consistent} with $M$ if
  for all literals $L = [\neg] P(a_1,\ldots,a_n)$ of opposite sign in $M$ we have
  $M\models \vee_{i\in I} \; a_i\neq b_i$ where $I$ contains exactly the indexes of
  syntactically different constants between  $P(b_1,\ldots,b_n)$ and $P(a_1,\ldots,a_n)$.
  We say that a trail $M$ is \emph{strongly consistent} if for every decomposition
  $M =M',L,M''$ $L$ is strongly consistent in $M'$.
\end{definition}

% \bigskip
% \shortrules{Fail}
% {$(M;N;U;B;k;\top$}
% {$(M;N;U;B;-1;\bot)$}
% { provided there is a constrained clause $\Lambda\|\bot\in N\cup U$
% and a simple ground substitution $\sigma$ \st $\models_\B\Lambda\sigma$
% }{\SCLT}{11}
%   \bigskip
%   \shortrules{Backtrack}
%   {$(M,K^{i+1},M';N;U;B;k;(\Lambda\| D)\cdot\sigma)$}
%   {$(M,M'';N;U\cup\{\Lambda\| D\};B;i;\top)$}
%   { provided $D=D'\lor L$ where $L\sigma$ is of level $k$ and $D'\sigma$ is of level $i$
%   and $M'' = \Lambda\sigma,L\sigma^{\Lambda\|D'\lor L\cdot\sigma}$ or $D=\bot$, $i=0$, and $M'' = \epsilon$
% }{\SCLT}{11}

% \begin{lemma}
% Let $N$ be an unsatisfiable set of pure constrained clauses.
% Then unsatisfiability of $N$ can be derived by $\SCLT$.
% \end{lemma}
% \begin{proof}
% If $N$ is unsatisfiable it can be decided by hierarchic superposition which is refutationally complete on pure constrained clause sets.
% Since hierarchic superposition can be simulated using first order resolution. Here we only need to show that we can simulate resolution steps acting on first order literals and not involving tautologies. This can be proved in a fashion similar to \cite{FioriWeidenbach19}.
% \end{proof}

\bigskip
\shortrules{Decide}
{$(M;N;U;B;k;\top)$}
{$(M,\Phi^{k+1},L^{k+1};N;U;B;k+1;\top)$}
{provided $N^{\mathcal B}\cup U^{\mathcal B}\cup M^{\mathcal B}\cup\Phi$ is $\mathcal T^{\mathcal B}$-satisfiable,
  $L\sigma$ is undefined in $M$, $|L|$ occurs in $N\cup U$ and $\cdom(\sigma)\subseteq B$,
  and $\Phi$ is a CNF of negated equalities $(\bigwedge_l\bigvee_i a_{li}\neq b_{li})$ such that $M,\Phi,L$ is strongly consistent
}{\SCLT}{12}

\bigskip
\shortrules{Propagate}
{$(M;N;U;B;k;\top)$}
%{$(M, \gamma_1\sigma,\dots,\gamma_n\sigma,L\sigma^{\Lambda\| C\lor L\cdot\sigma};N;U;B;k;\top)$}
{$(M, \Lambda\sigma^{\Lambda\| C\lor L\cdot\sigma},L\sigma^{\Lambda\| C\lor L\cdot\sigma};N;U;B;k;\top)$}
{provided $\Lambda\| C\lor L\in N\cup U$, $N^{\mathcal B}\cup U^{\mathcal B}\cup M^{\mathcal B}\cup\Lambda\sigma$
  is $\mathcal T^{\mathcal B}$-satisfiable, $\sigma$ is simple and ground,
  $M\models\lnot(C)\sigma$, $\cdom(\sigma)\subseteq B$, and $L\sigma$ is undefined in $M$
}{\SCLT}{12}

\bigskip
\shortrules{Conflict}
{$(M;N;U;B;k;\top)$}
{$(M;N;U;B;k;\Lambda\| D\cdot\sigma)$}
{provided $\Lambda\|D\in N\cup U$, $N^{\mathcal B}\cup U^{\mathcal B}\cup M^{\mathcal B}\cup\Lambda\sigma$ is $\TB$-satisfiable,
  $\sigma$ is simple and ground, $M\models\lnot(D)\sigma$, $\cdom(\sigma)\subseteq B$
}{\SCLT}{12}

\bigskip
\shortrules{Fail}
{$(M;N;U;B;k;\top)$}
{$(M;N;U;B;-1;\bot)$}
{provided there are clauses $\Lambda_1\|\bot,\dots,\Lambda_n\|\bot\in N\cup U$
  such that $\Lambda_1\|\bot,\dots,\Lambda_n\|\bot\models_{\B}\bot$
}{\SCLT}{12}

\bigskip
\shortrules{Backtrack}
{$(M,K^{i+1},M';N;U;B;k;(\Lambda\| D)\cdot\sigma)$}
{$(M,M'';N;U\cup\{\Lambda\| D\};B;i;\top)$}
{provided $D=D'\lor L$ where $L\sigma$ is of level $k$ and $D'\sigma$ is of level $i$
  and $M'' = \Lambda\sigma,L\sigma^{\Lambda\|D'\lor L\cdot\sigma}$ or $D=\bot$, $i=0$, and $M'' = \epsilon$
}{\SCLT}{11}

\begin{theorem}\label{thm:non-sub}
  Let $N$ be a set of constrained clauses.
  Then clauses learned in a {\SCLT} regular run
  (with the addition of also rule Grow)
  from starting state $(\epsilon;N;\emptyset;B;0;\top)$ are not subsumed.
\end{theorem}
\begin{proof}
Consider the following fragment of a derivation learning a clause:\newline
  \centerline{$\Rightarrow^{{Conflict}}_{\text{\SCLT}}(M;N;U;B;k;\Lambda_0\|C_0\cdot\sigma_0) \Rightarrow^{\{\text{Skip, Fact., Res.}\}^*}_{{\SCLT}} (M';N;U;B;k;\Lambda\|C\cdot\sigma)\Rightarrow^{\text{Backtrack}}_{{\SCLT}}.$}
  By soundness of resolution $N\cup U \models \Lambda\|C$
  and $\Lambda\sigma\|C\sigma$ is false under both $M$ and $M'$.
  We prove that $\Lambda\sigma\|C\sigma$ is not subsumed in $N\cup U$.

  Since the set of available arithmetic constants $B$
  can only increase during the derivation we can assume
  that every arithmetic constant appearing in
  $(M;N;U;B;k;\Lambda_0\|C_0\cdot\sigma_0)$ is in $B$.
  Since all literals and clauses needed for this proof
  are obtained from literals and clauses appearing in
  $(M;N;U;B;k;\Lambda_0\|C_0\cdot\sigma_0)$ and
  by combining them with normal operations and unification
  we never run the risk of exhausting the set $B$ of constants
  during conflict resolution.
  Indeed computing the $\mMGU$ between literals or constrained clauses
  never requires introducing new constants.

  Assume there is a $D \in \mGnd_B(N\cup U)$
  \st $D$ subsumes $\Lambda\sigma\|C\sigma$.
  As $\Lambda\sigma\|C\sigma$
  is false under $M$ we also have
  that $D$ must be false under $M$.

  Let $M''$ be the difference between $M'$ and $M$,
  that is $M = M',M''$, we distinguish two cases
  depending on whether $M''$
  contains or not any first order literal.

  If $M''$ contain a first order literal then $\Lambda\sigma\|C\sigma$ does
  not contain the rightmost first order literal of $M$ and
  since $D\subseteq \Lambda\sigma\|C\sigma$ neither does $D$.
  So at a previous point in the derivation there must have been
  a state such that $D$ was false under
  the current trail but was not chosen as conflict
  instance, a contradiction to the exhaustive
  application of Conflict.

  If $M''$ contains no first order literals
  then the rightmost first-order literal $L$ of $M$
  is in $M'$. Without loss of generality we assume
  that conflict resolution start with enough Skip
  applications to reach the trail $M_0=M_1,L$.
  We distinguish two sub-cases
  according to whether $L$% the rightmost literal in $M$
  is the result of a Decision or a Propagation.

  If the rightmost literal of $M_0=M_1,L^k$ is a
  decision literal, then $D$ must be false under
  $M_0$ and undefined under $M_1$.
  Moreover since Propagation has precedence over Decision
  we know $D$ has at least two undefined first order
  literals of level $k$. By the precondition of Backtrack
  we know that $C\sigma$  has at most one literal of level $k$
  in contradiction with $D\subseteq C\sigma$.

  If $M_0=M_1,L^{\Lambda'\|C'\cdot\delta}$ then we distinguish
  whether $C$ is empty of not.
  If $C=\bot$ we must also have $D=\Lambda''\|\bot$.
  By the preconditions on Conflict we have that
  $D\cup M^{\mathcal B}$ is satisfiable, we also have
  that $\Lambda\sigma\subseteq M^{\mathcal B}$, a contradiction
  as $\Lambda''\subseteq\Lambda\sigma$.

  If $C\neq\bot$ then exactly one literal in $C\sigma$ is of level
  $k$ and all other literals, if any, are of level at most $k-1$.
  Moreover, $D$ must have two literals of level $k$ that are falsified by $M_0$.
  % Backtrack requires the presence of at least one decision literal on the trail
  % and so $k > 0$ so $D$ must have at least two literals of level $k$.
  If both of those literal are different from $\comp(L)$ then by regularity,
  we would have applied Conflict on the trail instead of Propagate on the trail $M_1$.
  So at least one of the literals of level $k$ in $D$ must be $\comp(L)$.
  So $D$ cannot subsume $C\sigma$ as it has either one literal of level $k$
  that does not appear in $C\sigma$ or contains $L$
  with a higher multiplicity than $C\sigma$.
\end{proof}

With only Theorem \ref{thm:non-sub} and no conditions on the use of Factorize it is not possible
to give a simple \textit{a priori} bound to the number of clauses that can be
learned in a regular run, we can only prove that it must be finite.

\begin{theorem}[Decision Procedure on Ground Clauses]
  $\SCLT$ restricted to regular runs is a decision
  procedure for pure ground clause sets.
\end{theorem}
\begin{proof}
  Since in $N$ there are neither variables nor
  foreground constants of background sorts
  we can assume that all arithmetic terms in $N$ are numerical literals
  so that for two arithmetic terms $s$, $t$ we have
  $N\models_{\mathcal B}s=t$ if and only if $\models s=t$.
  In particular this means that we can keep
  clauses in $N$ unabstracted.

  If $N$ is ground it is enough to define $B$ as the set
  of all constants appearing in $N$.
  We need to prove that $\SCLT$ never get stuck without either reaching
  the sentinel state $(M;N;U;B;k;\Lambda\|\bot\cdot\sigma)$ or
  building and explicit model $M\models_BN$.
  Since conflict resolution can never get stuck
  we consider a conflict search state $(M;N;U;B;k;\top)$
  at which a regular run started at
  $(\epsilon;N;\emptyset;B;k;\top)$ terminates.
  If at the state $(M;N;U;B;k;\top)$ the rules
  Propagate, Decide, and Conflict cannot be applied
  it means that all first order literals in $N$ are
  defined in $M$ and that all constrained clauses
  $\Lambda\|C$ either have unsatisfiable constraints
  or have some literals defined true.
  This means that $M$ is a partial model of $N$.
\end{proof}
